# Supplementary material for: Dark Energy Survey Year 3 results: curved-sky weak lensing mass map reconstruction
Source: arXiv:2105.13539 source file (2021-11-22)
Supplement: Supplementary file 1 [file Appendix.tex]

% \section{Author Affiliations}
% \label{sec:affiliations}
% {\small
% $^{1}$ Laboratoire de Physique de l'Ecole Normale Sup\'erieure, ENS, Universit\'e PSL, CNRS, Sorbonne Universit\'e, Universit\'e de Paris, Paris, France
% $^{2}$ Department of Physics \& Astronomy, University College London, Gower Street, London, WC1E 6BT, UK
% $^{3}$ 
% }

% %

% %We show in Fig.~\ref{fig:svy1} the maps obtained in the DES Y1 and SV footprint, smoothed at 10 arcminutes. These maps have been obtained from other catalogues and photo-$z$ codes (SV used \texttt{ngmix} for the shape estimation and SKYNET for the photo-$z$ estimates; DES Y1 used \texttt{METACALIBRATION} and BPZ). The SV map is also half a magnitude deeper than the Y1 and Y3 maps, which have similar depths. Visually, the three maps agree in the region where their footprint overlaps, constituting a good consistency check between the different catalogues.

% { 
% \section{Alternative samples of voids}
% \label{sec:AppVoids}
% We considered alternative catalogues of voids to test how the mass map imprints may depend on the void definition and selection. 

% \texttt{VIDE}\footnote{https://bitbucket.org/cosmicvoids/} \citep{videpaper} is a watershed void finder based on \texttt{ZOBOV} \citep{neyrinck} that has been widely employed for various void studies \citep[see e.g.][and references therein]{Hamaus2020}. It has already been successfully used to study voids in the DESY1 data \citep{Pollina2019, Fang2019}.

% \texttt{VIDE}'s default centre is the volume-weighted barycentre, which does not generally coincide with the density minimum inside the void due to non-spherical void geometry. Instead, the barycentre preserves information about the void boundary. Therefore, a different kind of imprint signal is expected when correlated with convergence maps, with more pronounced positive rings rather than negative centres \citep[see][for a comprehensive study on the $\kappa$ signal associated with voids]{Cautun2016}. In the DES Y3 redMaGiC data, \texttt{VIDE} detected $12,841$ voids. We then halved this catalogue using the \textit{compensation} of voids to further increase and isolate the expected signal from the boundary zone, expecting to see an enhanced positive convergence $\kappa$ imprint from these over-compensated voids.

% \begin{figure}
% \begin{center}
% \includegraphics[width=86mm]{figures/massmap_KS_2D_newerrors_4panels_allmaps_unblinded.pdf}
% \end{center}
% \caption{The top panel illustrates the different mass map imprints of different types of voids. The lower panels show differences in signals measured from different mass map reconstructions, relative to the KS results and errors (shaded ranges are $1\sigma$ and $2\sigma$ around the KS results).  {\NJ{The figure needs the teX font to match the text}}}
% \label{fig:void_profile_more}
% \end{figure}

% We are also interested in detecting the most pronounced negative $\kappa$ signals associated with a specific subclass of large and deep voids that are \emph{under}-compensated. As a third option, we thus used the public\footnote{https://github.com/seshnadathur/REVOLVER/} void finder algorithm \texttt{REVOLVER} \citep{Nadat2018,beyondbao}, also based on the \texttt{ZOBOV} algorithm.

% A proxy for the gravitational potential (and thus for the convergence field) at the positions of voids can be defined as
% \begin{equation}
% \label{eq:lambda_v}
% \lambda_v\equiv\overline\delta_g\left(\frac{R_{\rmn{eff}}}{1\;h^{-1}\rmn{Mpc}}\right)^{1.2} \ \ ,
% \end{equation}
% using the average galaxy density contrast $\overline\delta_g = \frac{1}{V}\int_{V}\delta_g\,\rmn{d}^3\mathbf{x}$ and the effective spherical radius, $R_\rmn{eff}= \left(\frac{3}{4\pi}V\right)^{1/3}$, where the volume $V$ is the total volume of the void \citep[see][for further details]{NadathurCrittenden2016,Nadathur2017}. 
% \cite{cmbboss} showed that different values of the $\lambda_{v}$ parameter indicate different (CMB) lensing imprints, including signals with either positive or negative sign, aligned with the void centre\footnote{\texttt{REVOLVER} voids may also be defined using barycentres.}. Following this, we keep only $7,782$ of  the most under-compensated voids defined by the lowest $\lambda_{v}$ values. Leaving more detailed analyses for future work, we note that a subclass of voids with high $\lambda_{v}$ values would also correspond to over-compensated voids such as our \texttt{VIDE} sample.

% Fig.~\ref{fig:void_profile_more} shows the measured profiles of our \texttt{REVOLVER}, \texttt{VIDE}, and 2D void analyses given the uncertainties. As anticipated based on the differences in the nature of the voids we selected, we detected qualitatively different signals in each case:
% \begin{itemize}
% \item the \texttt{VIDE} voids show a relative depression in convergence at the void centre compared to the pronounced peak at the void boundary, matching our expectations.
% \item the \texttt{REVOLVER} voids we selected are associated with strong negative $\kappa$ imprints that in fact extend far beyond the void radius, indicating surrounding voids on average.
% \item 2D voids combine the advantages of the other finders. They excel in marking the actual radius of voids in the mass map profiles, with reduced central and wall amplitudes.
% \end{itemize}

% We thus report that all three void types we consider show consistent signals when mass maps are varied for a given void sample. We leave more detailed analysis for future work.}
